# Supplementary material for: PoLLMgraph: Unraveling Hallucinations in Large Language Models via State Transition Dynamics
Source: arXiv:2404.04722 source file (2024-04-06)
Supplement: Supplementary file 1 [file appendix_bka.tex]

\newpage
\appendix
\section{Additional Method Details}
\subsection{State Abstraction}
\label{appendix:method:state_abstract}
The dimension of each initial state generated by LLMs is equal to the number of hidden units in the hidden layer of transformers, which is usually very high. It is hard to find the latent characteristics over high dimensional space since the distribution of data with high dimensions tends to be sparse~\cite{krishnan2018challenges}. Therefore, we first reduce the dimension of each initial state generated by the data generation to an optimal number automatically.  
Previous studies~\cite{du2019deepstellar} applied Principal Component Analysis (PCA) to reduce the dimension of semantic space to a small number, in order to find the common correlation over states efficiently. However, there exists an obvious limitation in their approach. When the dimension of an initial state is high, arbitrary dimension reduction may lead to a huge information loss. The information loss from modelling may introduce a high bias in the following semantic model construction potentially. To improve the semantic model construction, we use a classic metric, Related Error Rate, to measure the information loss during dimension reduction. In detail, we have a number of $n$ vector $V$ and each vector is with $m$-dimension space, i.e.,  $[v_0, v_1,...,v_m]$. We want to transform the $n$ initial vectors to vectors $\hat{V}$, and each transformed vector is with $k$ dimension, i.e., $[\hat{v}_0,\hat{v}_1, ..., \hat{v}_k]$. The corresponding information loss $\psi$ can be defined as:
\begin{equation}
    \psi(k) = \frac{1}{n} * \sum_{j=1}^{n} \frac{\sum_{i=1}^{k}(v_i^{j} - \hat{v}_i^j)^2}{\sum_{i=1}^{k}(v_i^j)^2}
\end{equation}
In order to overcome the aforementioned limitation, we take information loss into account for dimension reduction in order to secure the generalize of internal state transformation. We set a threshold $\theta$ to control information loss, and the decision process of finding the optimal $k$ can be defined as:
\begin{equation} 
    k \gets \argmin_{k} | \psi(k) - \theta| 
\end{equation}
Finally, this step outputs intermediate states and each state has $k$ dimensions. 

Given a $K$-dimensional state space $R^K$, the termination state $s$ is represented as $(s^0,...,s^{K-1})$. The value of the $i$-th dimension can be scaled into $[l_i,u_i]$, where the $l_i$ and $u_i$ are the lower and upper boundaries. We equally split the value scopes into $N$ intervals of each dimension. In this way, we convert the continuous state space into a discrete state space with finite grids on each dimension as follows: 
\begin{equation}
e_n^i=[l_i+n\times\frac{u_i-l_i}{N},l_i+(n+1)\times\frac{u_i-l_i}{N}]
\end{equation}
where different concrete termination states $s$, which are located in the same grid, will be assigned by a common and unique label $\hat{s}$ as follows:
\begin{equation}
\hat{s}=\{s|s^i\in{e_n^i},n\in[0,N-1],i\in[0,K-1]\}
\end{equation}
We apply grid-based clustering to transform the concrete termination states (extracted embeddings) into countable abstract states. Topologically similar concrete states will fall into the same grid as an abstract state. Each abstract state represents a cluster. 

An example of a grid-based state cluster in a 2-dimensional state space is shown in Figure~\ref{grid}. The figure demonstrates that several concrete states (i.e., points on the left) are clustered into three types of abstract states (i.e., clusters): abstract states \textit{4, 5, 9, 17, 20} with occurrences $\eta=1$, abstract state \textit{11} with occurrences $\eta=2$, and abstract state \textit{19} with occurrences $\eta=3$.

\begin{figure}[t!]
\centering
\includegraphics[width=0.45\textwidth]{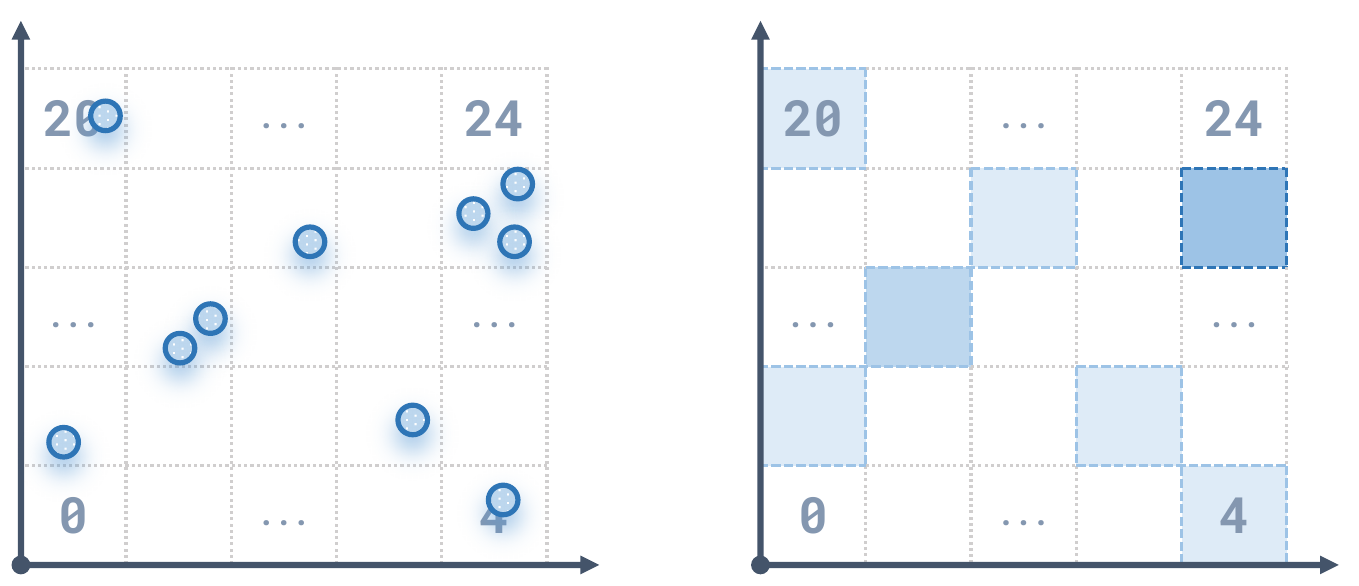}
\caption{The process of grid-based abstraction in 2-dimensional state space can be illustrated with a schematic diagram. The diagram on the left side depicts the specific termination states, while the right side represents the abstract states generated by grid-based clustering.}
\label{grid}
\end{figure}

\subsection{Hiiden Markov Model}
HMM~\cite{eddy1998profile,rabiner1986introduction}, is designed to catch the sequential dependencies in sequence data and is able to provide a probability distribution over possible sequences.
Hence, we also choose HMM to model the hidden state traces.

\begin{mydefinition}[\emph{Hidden Markov Model}]
    An HMM is a tuple $(\bar{S}, \bar{\delta}, \bar{P}, \bar{O}, \bar{E}, \bar{I})$, where $S$ is the hidden state space, $\bar{\delta}$ is the transition space, $\bar{P}: \bar{S} \times \bar{S} \rightarrow [0, 1]$ is the transition probability function that maps the transition to the probability distribution, $O = \{o_1, \dots, o_n\}$ is the finite set of observations, $E: (s_i, o_j) \rightarrow [0,1]$ is the emission function that maps the observation $o_j$ being generated from state $s_i$ to a probability distribution, and $I: S \rightarrow [0, 1]$ is the initial state probability function that map the state space to the probability distribution.
\end{mydefinition}

The construction of HMM is as follows. We first define the state space $S$ with the number of hidden states and the observations $O$. Moreover, we use the standard HMM fitting procedure -- Baum-Welch algorithm~\cite{} (as an Expectation-Maximization algorithm) to compute transition probability $P$, Emission function $E$, and initial state probability function $I$. Baum-Welch algorithm is composed of \emph{expectation}, which calculates the conditional expectation given observed traces, and \emph{maximization}, which updates the parameters of $P$, $E$, and $I$, to maximize the likelihood of observation.

\small
\begin{equation}
\begin{split}
    Pr(\text{failure}=1|O_{1}^{T}) & =   \sum_{S_{1}^{T}} Pr(\text{failure}=1,S_{1}^{T}|O_{1}^{T})) \\
& = \sum_{S_{1}^{T}}Pr(\text{failure}=1|S_{1}^{T})*Pr(S_{1}^{T}|O_{1}^{T}) \\
& \propto \sum_{S_{1}^{T}}[\frac{Pr(O_{1}^{T}|S_{1}^{T})}{Pr(O_{1}^{T})}\cdot Pr(S_{1}^{T}|\text{failure=1})]
\end{split}
\end{equation}

 \begin{itemize}
    \item \textbf{Step 1} state abstractions:
    \begin{itemize}
        \item extract embedding as concrete states
        \item transform concrete states to abstract states (PCA and clustering)
        \item generates the traces in terms of the abstract states and training data
    \end{itemize}
    \item \textbf{Step 2} Modeling the abstracted traces and apply the trace to detect hallucinations. 
\end{itemize}

\subsection{Additional experiments on distribution shift}

\section{Experiment Setup}
\subsection{Baseline Methods}
We conducted a thorough search of related work and made every effort to include all peer-reviewed, relevant works in our comparison for this paper, even those less directly comparable, such as hallucination rectification methods that permit an intermediate detection step. For all baseline methods, we used their open-source implementations to conduct the experiments when available. The only exception is "Uncertainty", which is not open-sourced and thus requires a straightforward reimplementation. We present a more detailed description of each baseline method in the following sections. The latent activation, internal state and ITI requires labelled reference data as training data. In the experiments, these apporaches use the same reference data as \texttt{PoLLMgraph}.

\paragraph{Uncertainty~\cite{xiao2021hallucination}.} This is to use the prediction distribution at each decoding step to calculate the entropy of generated text for evaluating the uncertainty of generated text. The uncertainty scores can be directly used for measuring the hallucinations. We conduct experiments on this baseline with our own implementation since there is no official open-source code released along with this method.

\paragraph{Latent Activation~\cite{burns2022discovering}.} This approach is to find out the pattern of direction in activation space for hallucination content. For each QA pair, we convert them to a yes/no question. Each QA pair follow with a yes and a no answer, in which \textit{yes} means hallucination and \textit{no} refers to non-hallucination. The groundtruth of each QA is automatically annotated by the fine-tuned GPT models. We use the official repository (\href{https://github.com/collin-burns/discovering_latent_knowledge}{https://github.com/collin-burns/discovering\_latent\_knowledge}) to conduct experiments.

\paragraph{Internal State~\cite{azaria-mitchell-2023-internal}.} This approach is to train a neural network-based classifier using the activation as input to predict whether the output of LLM is reliable. In our experiments, we annotate each QA pair whether the answer is hallucination. Then, we extract the activations of the last layer from the last token on each QA pair. The activations extracted from training data are used for training the classifier and the activations extracted from the rest data are used for evaluating the effectiveness of hallucination detection. We use the open-source code (\href{https://github.com/balevinstein/Probes}{https://github.com/balevinstein/Probes}) to conduct experiments.

\paragraph{ITI~\cite{li2023inference}.} Similar to the Internal State approach, ITI takes the activations as input to predict an intermediate detection score, which can be applied to detecting whether the output is hallucinations. The difference is that the ITI used a logistic regression model to predict, while Internal State used a simple three-layer-based feedforward neural network model. In this experiment, we extract the activations of the last layer from the last tokens on each QA pair. These activations are used for training the logistic model and evaluating the effectiveness of hallucination detection with annotated ground-truth. We use the intermediate detection scores, which are predicted by a logistic regression model, as the hallucination prediction scores. we use the official repository \href{https://github.com/likenneth/honest_llama}{https://github.com/likenneth/honest\_llama} to conduct experiments.

\subsection{Additional Experiments}
We further conduct experiments more baseline approach.

\begin{table*}[!t]
\aboverulesep=0ex
\belowrulesep=0ex
\newcommand{\cc}{\cellcolor{Gray}}
\resizebox{\textwidth}{!}{%
\begin{tabular}{l|c|cccc}
\toprule
\multicolumn{1}{c|}{\multirow{2}{*}{\textbf{Method Name}}}
 & \multicolumn{1}{c|}{\multirow{2}{*}{\textbf{Method Type}}}     &  \multicolumn{4}{c}{\textbf{Models}}\\
 \cline{3-6}
&  & Llama-13B & Alpaca-13B & Vicuna-13B & Llama2-13B \\
\midrule
SelfCheck-BERTScore   & black-box    &  0.55      & 0.52       & 0.51       & 0.54       \\
SelfCheck-MCQA    & black-box         &  0.52      & 0.51      & 0.52       & 0.54       \\
SelfCheck-Ngram     & black-box       &  0.65      & 0.60      & 0.59       & 0.61       \\
SelfCheck-Combination   & black-box   &  0.65      & 0.60      & 0.61       & 0.63       \\
SelfContradictory     & black-box     &  0.54      & 0.52      & 0.53       & 0.52       \\
Uncertainty         & gray-box      &  0.54      & 0.53        & 0.53       & 0.52       \\
ITI                   & white-box    &  0.67      & 0.64       & 0.62       & 0.64       \\
Latent Activations    & white-box    &  0.65      & 0.61       & 0.59       & 0.60       \\
Internal State    & white-box    &  0.67      & 0.64       & 0.65       & 0.67       \\
\cc PoLLMgraph-MM (Grid)        & \cc white-box    &   \cc  0.64  & \cc 0.67 & \cc 0.68 & \cc   0.69 \\
\cc PoLLMgraph-MM (GMM)        & \cc white-box    &   \cc 0.72    & \cc 0.73  & \cc 0.71 & \cc 0.73    \\
\cc PoLLMgraph-HMM (Grid)   & \cc white-box  & \cc 0.84    & \cc \textbf{0.86}       & \cc \textbf{0.84}    & \cc 0.87       \\
\cc PoLLMgraph-HMM (GMM) & \cc white-box & \cc \textbf{0.85}      & \cc 0.85     & \cc 0.83       & \cc \textbf{0.88}       \\
\bottomrule
\end{tabular}%
}
\caption{The detection \textbf{AUC-ROC} for different approaches over multiple benchmark LLMs. The ITI and Latent Activation uses the same reference data as \texttt{PoLLMgraph}. The \colorbox{Gray}{shaded area} illustrates our proposed variants of approaches. The best results are highlighted \textbf{in bold}.}
\label{tab:empirical_results_detection_overall}
\vspace{10pt}
\end{table*}
